# Supplementary material for: On the Statistical Relation of Ultra-Reliable Wireless and Location Estimation
Source: arXiv:2308.14416 source file (2023-08-28)
Supplement: Supplementary file 1 [file Fisher_appendix.tex]

The derivative of the mean of the normalized received signal at the $i$th \gls{bs} for the $j$th subcarrier, i.e$.$, $\mu_{i,j} = \sum_{k=1}^K a_{i, k} d_j(\Tilde{\tau}_{i, k})$, with respect to the unknown channel parameters is
\begin{align}
    \frac{\partial \mu_{i,j}}{\partial \tilde{\tau}_{i, k}} &= -a_{i, k} \jmath 2\pi j \Delta_f \exp(-\jmath2\pi j \Delta_f \Tilde{\tau}_{i, k}),\\
    \frac{\partial \mu_{i,j}}{\partial \mathfrak{R}(a_{i,k})} &= \exp(-\jmath2\pi j \Delta_f \Tilde{\tau}_{i, k}),\\
    \frac{\partial \mu_{i,j}}{\partial \mathfrak{I}(a_{i,k})} &= \jmath\exp(-\jmath2\pi j \Delta_f \Tilde{\tau}_{i, k}).
\end{align}
The Fisher information matrix is symmetric and can be expressed analytically as (assuming that $j=-N/2,\dots,N/2$)
\begin{equation}
    J(\mbs{\eta}_i) = \frac{8\pi P_{\text{tx}}}{N_0}
    \begin{pmatrix}
        \mbs{J}_{\mbs{\tau}_{i}} & \mbs{J}_{\mbs{\tau}_{i}\mbs{a}_{i}}^T \\
        \mbs{J}_{\mbs{\tau}_{i}\mbs{a}_{i}} & \mbs{J}_{\mbs{a}_{i}\mbs{a}_{i}}
    \end{pmatrix}
\end{equation}
where
\begin{align}
    [\mbs{J}_{\mbs{\tau}_{i}}]_{n,m} &= 4\pi \Delta_f
    \begin{cases}
        \mathfrak{R}(a_n a_m^*)\sum_{j=1}^{N/2} j^2 \mathfrak{R}(d_j(\tau_{i,n}-\tau_{i,m})), & n \neq m,\\
        |a_n|^2 \frac{N(N+1)(N+2)}{24}, & n = m,
    \end{cases}\\
    \mbs{J}_{\mbs{\tau}_{i}\mbs{a}_{i}} &= -
    \begin{pmatrix}
        \mbs{A}~\text{diag}(\mathfrak{R}(\mbs{a}_i))\\
        \mbs{A}~\text{diag}(\mathfrak{I}(\mbs{a}_i))
    \end{pmatrix},\\
    [\mbs{A}]_{n, m} &=
    \begin{cases}
        \sum_{j=1}^{N/2} j \mathfrak{I}(d_j(\tau_{i,n}-\tau_{i, m})), & n \neq m,\\
        0, & n = m,
    \end{cases}\\
    \mbs{J}_{\mbs{a}_{i}\mbs{a}_{i}} &=
    \begin{pmatrix}
        \mbs{J}_{\mathfrak{R}(\mbs{a}_{i})\mathfrak{R}(\mbs{a}_{i})} & \mbs{0}\\
        \mbs{0} & \mbs{J}_{\mathfrak{I}(\mbs{a}_{i})\mathfrak{I}(\mbs{a}_{i})}
    \end{pmatrix},\\
    [\mbs{J}_{\mathfrak{R}(\mbs{a}_{i})\mathfrak{R}(\mbs{a}_{i})}]_{n, m} &= [\mbs{J}_{\mathfrak{I}(\mbs{a}_{i})\mathfrak{I}(\mbs{a}_{i})}]_{n,m}\\
    &=
    \begin{cases}
        1 + 2 \sum_{j=1}^{N/2}\mathfrak{R}(d_j(\tau_{i, n} - \tau_{i, m})), & n \neq m,\\
        N + 1, & n = m.
    \end{cases}
\end{align}

% \big(-4\pi \Delta_f \text{diag}(\mathfrak{R}\{\mbs{a}_i\})\big)^T
% \big(-4\pi \Delta_f \text{diag}(\mathfrak{I}\{\mbs{a}_i\})\big)^T
